# Supplementary material for: Seq2Seq2Sentiment: Multimodal Sequence to Sequence Models for Sentiment Analysis
Source: arXiv:1807.03915 source file (2018-08-06)
Supplement: Supplementary file 1 [file appendix.tex]

\appendix
% \twocolumn[\section{Confusion matrix comparison between baseline and Seq2Seq bimodal models}]
\section{Confusion matrix comparison between baseline and Seq2Seq bimodal models} 
\label{sec:appendix_a}
Table \ref{tbl:multimodal_confusion} details the confusion matrix of our unimodal and bimodal results. 
%------------------------------------------------------------------------
\begin{table*}
\begin{center}
\begin{tabular}{l|c|c|ccc|ccc|c}
\multicolumn{3}{c}{} & \multicolumn{3}{c}{\textbf{Baseline}} & \multicolumn{3}{c}{\textbf{Seq2Seq}} & No. \\ %\cline{4-9}
{Modalities} & {Setting} & {Class} & \multicolumn{1}{l}{Prec} & \multicolumn{1}{l}{Recall} & \multicolumn{1}{l}{F1} & \multicolumn{1}{l}{Prec} & \multicolumn{1}{l}{Recall} & \multicolumn{1}{l}{F1} & Samples \\
\toprule
% 1
\centering
\multirow{11}{*}{Text+Audio} & 
	\multirow{3}{*}{Binary} & 
    	\multicolumn{1}{l}{0} & \multicolumn{1}{l}{{0.66}} & \multicolumn{1}{l}{{1.00}} & \multicolumn{1}{l}{{0.80}} & \multicolumn{1}{l}{{0.74}} & \multicolumn{1}{l}{{0.61}} & \multicolumn{1}{l}{{0.67}} & \multicolumn{1}{l}{{453}}\\
        & {} & 
        \multicolumn{1}{l}{1} & \multicolumn{1}{l}{{0}} & \multicolumn{1}{l}{{0}} & \multicolumn{1}{l}{{0}} & \multicolumn{1}{l}{{0.44}} & \multicolumn{1}{l}{{0.59}} & \multicolumn{1}{l}{{0.50}} & \multicolumn{1}{l}{{233}}\\
        & {} & 
        \multicolumn{1}{l}{AVG.} & \multicolumn{1}{l}{{0.44}} & \multicolumn{1}{l}{{0.66}} & \multicolumn{1}{l}{{0.53}} & \multicolumn{1}{l}{{0.64}} & \multicolumn{1}{l}{{0.60}} & \multicolumn{1}{l}{{0.61}} & \multicolumn{1}{l}{{686}}\\
        \cline{2-{10}}
    & 
    \multirow{8}{*}{7 Classes} & 
    \multicolumn{1}{l}{-3} & \multicolumn{1}{l}{{0}} & \multicolumn{1}{l}{{0}} & \multicolumn{1}{l}{{0}} & \multicolumn{1}{l}{{0}} & \multicolumn{1}{l}{{0}} & \multicolumn{1}{l}{{0}} & \multicolumn{1}{l}{{46}}\\
    & {} & 
    \multicolumn{1}{l}{-2} & \multicolumn{1}{l}{{0}} & \multicolumn{1}{l}{{0}} & \multicolumn{1}{l}{{0}} & \multicolumn{1}{l}{{0.24}} & \multicolumn{1}{l}{{0.18}} & \multicolumn{1}{l}{{0.21}} & \multicolumn{1}{l}{{156}}\\
	& {} & 
    \multicolumn{1}{l}{-1} & \multicolumn{1}{l}{{0}} & \multicolumn{1}{l}{{0}} & \multicolumn{1}{l}{{0}} & \multicolumn{1}{l}{{0.20}} & \multicolumn{1}{l}{{0.17}} & \multicolumn{1}{l}{{0.18}} & \multicolumn{1}{l}{{145}}\\
    & {} & 
    \multicolumn{1}{l}{0} & \multicolumn{1}{l}{{0.15}} & \multicolumn{1}{l}{{1}} & \multicolumn{1}{l}{{0.27}} & \multicolumn{1}{l}{{0.16}} & \multicolumn{1}{l}{{0.20}} & \multicolumn{1}{l}{{0.18}} & \multicolumn{1}{l}{{106}}\\
    & {} & 
    \multicolumn{1}{l}{1} & \multicolumn{1}{l}{{0}} & \multicolumn{1}{l}{{0}} & \multicolumn{1}{l}{{0}} & \multicolumn{1}{l}{{0.17}} & \multicolumn{1}{l}{{0.26}} & \multicolumn{1}{l}{{0.20}} & \multicolumn{1}{l}{{113}}\\
    & {} & 
    \multicolumn{1}{l}{2} & \multicolumn{1}{l}{{0}} & \multicolumn{1}{l}{{0}} & \multicolumn{1}{l}{{0}} & \multicolumn{1}{l}{{0.21}} & \multicolumn{1}{l}{{0.30}} & \multicolumn{1}{l}{{0.25}} & \multicolumn{1}{l}{{100}}\\
    & {} & 
    \multicolumn{1}{l}{3} & \multicolumn{1}{l}{{0}} & \multicolumn{1}{l}{{0}} & \multicolumn{1}{l}{{0}} & \multicolumn{1}{l}{{1}} & \multicolumn{1}{l}{{0.05}} & \multicolumn{1}{l}{{0.10}} & \multicolumn{1}{l}{{20}}\\
    & {} & 
    \multicolumn{1}{l}{AVG.} & \multicolumn{1}{l}{{0.02}} & \multicolumn{1}{l}{0.15} & \multicolumn{1}{l}{{0.04}} & \multicolumn{1}{l}{{0.21}} & \multicolumn{1}{l}{{0.20}} & \multicolumn{1}{l}{{0.19}} & \multicolumn{1}{l}{{686}}\\
    
\midrule
% 2 
\multirow{11}{*}{Text+Video} & 
	\multirow{3}{*}{Binary} & 
    	\multicolumn{1}{l}{0} & \multicolumn{1}{l}{{0.67}} & \multicolumn{1}{l}{{1.00}} & \multicolumn{1}{l}{{0.80}} & \multicolumn{1}{l}{{0.75}} & \multicolumn{1}{l}{{0.75}} & \multicolumn{1}{l}{{0.75}} & \multicolumn{1}{l}{{453}}\\
        & {} & 
        \multicolumn{1}{l}{1} & \multicolumn{1}{l}{{1}} & \multicolumn{1}{l}{{0.03}} & \multicolumn{1}{l}{{0.05}} & \multicolumn{1}{l}{{0.51}} & \multicolumn{1}{l}{{0.52}} & \multicolumn{1}{l}{{0.52}} & \multicolumn{1}{l}{{233}}\\
        & {} & 
        \multicolumn{1}{l}{AVG.} & \multicolumn{1}{l}{{0.78}} & \multicolumn{1}{l}{{0.67}} & \multicolumn{1}{l}{{0.55}} & \multicolumn{1}{l}{{0.67}} & \multicolumn{1}{l}{{0.67}} & \multicolumn{1}{l}{{0.67}} & \multicolumn{1}{l}{{686}}\\
        \cline{2-{10}}
    & 
    \multirow{8}{*}{7 Classes} & 
    \multicolumn{1}{l}{-3} & \multicolumn{1}{l}{{0}} & \multicolumn{1}{l}{{0}} & \multicolumn{1}{l}{{0}} & \multicolumn{1}{l}{{0.57}} & \multicolumn{1}{l}{{0.09}} & \multicolumn{1}{l}{{0.15}} & \multicolumn{1}{l}{{46}}\\
    & {} & 
    \multicolumn{1}{l}{-2} & \multicolumn{1}{l}{{0}} & \multicolumn{1}{l}{{0}} & \multicolumn{1}{l}{{0}} & \multicolumn{1}{l}{{0.22}} & \multicolumn{1}{l}{{0.12}} & \multicolumn{1}{l}{{0.15}} & \multicolumn{1}{l}{{156}}\\
	& {} & 
    \multicolumn{1}{l}{-1} & \multicolumn{1}{l}{{0}} & \multicolumn{1}{l}{{0}} & \multicolumn{1}{l}{{0}} & \multicolumn{1}{l}{{0.23}} & \multicolumn{1}{l}{{0.26}} & \multicolumn{1}{l}{{0.24}} & \multicolumn{1}{l}{{145}}\\
    & {} & 
    \multicolumn{1}{l}{0} & \multicolumn{1}{l}{{0.16}} & \multicolumn{1}{l}{{1}} & \multicolumn{1}{l}{{0.27}} & \multicolumn{1}{l}{{0.20}} & \multicolumn{1}{l}{{0.37}} & \multicolumn{1}{l}{{0.25}} & \multicolumn{1}{l}{{106}}\\
    & {} & 
    \multicolumn{1}{l}{1} & \multicolumn{1}{l}{{0}} & \multicolumn{1}{l}{{0}} & \multicolumn{1}{l}{{0}} & \multicolumn{1}{l}{{0.17}} & \multicolumn{1}{l}{{0.22}} & \multicolumn{1}{l}{{0.19}} & \multicolumn{1}{l}{{113}}\\
    & {} & 
    \multicolumn{1}{l}{2} & \multicolumn{1}{l}{{0.50}} & \multicolumn{1}{l}{{0.03}} & \multicolumn{1}{l}{{0.06}} & \multicolumn{1}{l}{{0.33}} & \multicolumn{1}{l}{{0.28}} & \multicolumn{1}{l}{{0.30}} & \multicolumn{1}{l}{{100}}\\
    & {} & 
    \multicolumn{1}{l}{3} & \multicolumn{1}{l}{{0}} & \multicolumn{1}{l}{{0}} & \multicolumn{1}{l}{{0}} & \multicolumn{1}{l}{{0.50}} & \multicolumn{1}{l}{{0.10}} & \multicolumn{1}{l}{{0.17}} & \multicolumn{1}{l}{{20}}\\
    & {} & 
    \multicolumn{1}{l}{AVG.} & \multicolumn{1}{l}{{0.10}} & \multicolumn{1}{l}{0.16} & \multicolumn{1}{l}{{0.05}} & \multicolumn{1}{l}{{0.26}} & \multicolumn{1}{l}{{0.22}} & \multicolumn{1}{l}{{0.22}} & \multicolumn{1}{l}{{686}}\\
    
\midrule
% 3
\multirow{11}{*}{Audio+Video} & 
	\multirow{3}{*}{Binary} & 
    	\multicolumn{1}{l}{0} & \multicolumn{1}{l}{{0.66}} & \multicolumn{1}{l}{{0.42}} & \multicolumn{1}{l}{{0.51}} & \multicolumn{1}{l}{{0.76}} & \multicolumn{1}{l}{{0.67}} & \multicolumn{1}{l}{{0.71}} & \multicolumn{1}{l}{{453}}\\
        & {} & 
        \multicolumn{1}{l}{1} & \multicolumn{1}{l}{{0.34}} & \multicolumn{1}{l}{{0.58}} & \multicolumn{1}{l}{{0.43}} & \multicolumn{1}{l}{{0.48}} & \multicolumn{1}{l}{{0.58}} & \multicolumn{1}{l}{{0.52}} & \multicolumn{1}{l}{{233}}\\
        & {} & 
        \multicolumn{1}{l}{AVG.} & \multicolumn{1}{l}{{0.55}} & \multicolumn{1}{l}{{0.47}} & \multicolumn{1}{l}{{0.48}} & \multicolumn{1}{l}{{0.66}} & \multicolumn{1}{l}{{0.64}} & \multicolumn{1}{l}{{0.65}} & \multicolumn{1}{l}{{686}}\\
        \cline{2-{10}}
    & 
    \multirow{8}{*}{7 Classes} & 
    \multicolumn{1}{l}{-3} & \multicolumn{1}{l}{{0}} & \multicolumn{1}{l}{{0}} & \multicolumn{1}{l}{{0}} & \multicolumn{1}{l}{{0.50}} & \multicolumn{1}{l}{{0.02}} & \multicolumn{1}{l}{{0.04}} & \multicolumn{1}{l}{{46}}\\
    & {} & 
    \multicolumn{1}{l}{-2} & \multicolumn{1}{l}{{0.13}} & \multicolumn{1}{l}{{0.01}} & \multicolumn{1}{l}{{0.02}} & \multicolumn{1}{l}{{0.33}} & \multicolumn{1}{l}{{0.12}} & \multicolumn{1}{l}{{0.18}} & \multicolumn{1}{l}{{156}}\\
	& {} & 
    \multicolumn{1}{l}{-1} & \multicolumn{1}{l}{{0.22}} & \multicolumn{1}{l}{{0.14}} & \multicolumn{1}{l}{{0.18}} & \multicolumn{1}{l}{{0.24}} & \multicolumn{1}{l}{{0.30}} & \multicolumn{1}{l}{{0.27}} & \multicolumn{1}{l}{{145}}\\
    & {} & 
    \multicolumn{1}{l}{0} & \multicolumn{1}{l}{{0.17}} & \multicolumn{1}{l}{{0.28}} & \multicolumn{1}{l}{{0.21}} & \multicolumn{1}{l}{{0.23}} & \multicolumn{1}{l}{{0.36}} & \multicolumn{1}{l}{{0.28}} & \multicolumn{1}{l}{{106}}\\
    & {} & 
    \multicolumn{1}{l}{1} & \multicolumn{1}{l}{{0.15}} & \multicolumn{1}{l}{{0.52}} & \multicolumn{1}{l}{{0.23}} & \multicolumn{1}{l}{{0.23}} & \multicolumn{1}{l}{{0.35}} & \multicolumn{1}{l}{{0.28}} & \multicolumn{1}{l}{{113}}\\
    & {} & 
    \multicolumn{1}{l}{2} & \multicolumn{1}{l}{{0}} & \multicolumn{1}{l}{{0}} & \multicolumn{1}{l}{{0}} & \multicolumn{1}{l}{{0.25}} & \multicolumn{1}{l}{{0.27}} & \multicolumn{1}{l}{{0.26}} & \multicolumn{1}{l}{{100}}\\
    & {} & 
    \multicolumn{1}{l}{3} & \multicolumn{1}{l}{{0}} & \multicolumn{1}{l}{{0}} & \multicolumn{1}{l}{{0}} & \multicolumn{1}{l}{{1}} & \multicolumn{1}{l}{{0.33}} & \multicolumn{1}{l}{{0.01}} & \multicolumn{1}{l}{{15}}\\
    & {} & 
    \multicolumn{1}{l}{AVG.} & \multicolumn{1}{l}{{0.13}} & \multicolumn{1}{l}{0.16} & \multicolumn{1}{l}{{0.11}} & \multicolumn{1}{l}{{0.28}} & \multicolumn{1}{l}{{0.25}} & \multicolumn{1}{l}{{0.23}} & \multicolumn{1}{l}{{686}}\\  
\bottomrule
\end{tabular}
\end{center}
\caption{Confusion matrix comparison between bimodal baseline model and our bimodal Seq2Seq model. Our modal significantly outperforms the baseline, especially in the 7-class case.}
\label{tbl:multimodal_confusion}
\end{table*}
